# Supplementary material for: Layout Sequence Prediction From Noisy Mobile Modality
Source: arXiv:2310.06138 source file (2023-10-09)
Supplement: Supplementary file 1 [file appendix.tex]

\clearpage
\appendix

\section{Dataset}
\label{app:dataset}
\subsection{Vi-Fi Multi-modal Dataset~\cite{liu2022vi,liu2021lost}.}
Vi-Fi is a large-scale multi-modal dataset for vision-wireless systems that aims to associate moving pedestrians and objects across RGB-D vision and wireless sensors. It leverages smartphone wireless data, including WiFi Fine Timing Measurements (FTM) for measuring the distance between the smartphone and the wireless receiver, and inertial measurement unit (IMU) sensors for capturing users' specific force, angular rate, and orientation using a combination of accelerometers, gyroscopes, and magnetometers. Additionally, it includes RGB-D images with object trajectories and bounding boxes in the camera footage, along with their corresponding smartphone identifiers. The Vi-Fi dataset contains 90 sequences (each lasting 3 minutes) of multimodal data, including indoor scenarios with five legitimate users and no passersby, and outdoor scenarios with 2-3 actual users and up to 12 passersby in view.

In the Vi-Fi dataset, we directly use the mobile signals collected from pedestrians and the bounding box and depth information from surveillance cameras as the visual modality. We calculate the Mean Squared Error per Timestamps (MSE-T) and Intersection over Union of Depth (IoU-D) as metrics to evaluate this dataset.

\subsection{H3D Dataset~\cite{360LiDARTracking_ICRA_2019}}
The Honda 3D dataset (H3D) is a large-scale, full-round dataset for autonomous driving. It has been widely used as a 3D multi-object detection and object tracking dataset. The data are originally from the HDD dataset~\cite{ramanishka2018CVPR}, a challenging naturalistic driving dataset for learning driver behavior in real-life environments. The dataset was collected in the San Francisco Bay Area using a car equipped with various sensors, including LiDAR, GPS, IMU, and cameras. It comprises 104 hours of real human driving videos, 1.7 billion 3D bounding box labels, eight common class labels annotated by humans, and a linear propagation algorithm at 10 Hz.

Since the annotated objects with 3D bounding boxes lack mobile modality data, we treat the vehicle collecting the data as the object with both visual and mobile modalities. In our experiments, we use the yaw angle, velocity, GPS, and IMU data as the mobile modality and odometry data as the visual modality. Because there is no 3D bounding box as layout information for the target object to calculate IoU-D, we use 3D odometry data as layout information but only use the Mean Squared Error per Timestamps (MSE-T) as evaluation metrics.
